# Supplementary material for: A numerical damped oscillator approach to constrained Schr\"{o}dinger equations
Source: arXiv:2002.04400 ancillary file (2020-10-20)
Supplement: Supplementary file 1 [file DFPM_1D_HO.pdf]

```
%
% DFPM_1D_HO.m % Supplemental material to M. \"{O}gren and M. Gulliksson, Eur. J.↙
Phys. 41 (2020) 065406.
% 1D Harmonic oscillator, corresponding to \omega=\hbar=m=1.
%
clear all; close all
tic;
%
% Number of orthonormalized wavefunctions to calculate.
max_nof_wf = 10; % 1,2,3,4, ...
%
% Damping parameters for DFPM, and for all constraints.
eta = 2; k = 2;
%
% Numerical tolerance and maximum number of iterations for the DFPM iteration.
tol = 1e-13; itermax = 1e6;
%
% Time step of the fictious time.
dtau = 0.05;
%
% Spatial discretization.
x_min = -8; x_max = -x_min; nof_x = 1e2;
x = linspace(x_min, x_max, nof_x); dx = x(2) - x(1);
%
% Harmonic oscillator potential.
V = 0.5*x.^2;
%
% Setting up the matrix H, the discrete representation of the Hamiltonian operator↙
\hat{H}.
H=1./dx^2*(spdiags([-0.5*ones(nof_x,1) ones(nof_x,1)+dx^2*V' -0.5*ones(nof_x,1)], ...
    -1:1, nof_x, nof_x) );
%
% Random initial condition for the wavefunction.
u_ini = -0.5+rand(length(x),1);
%
% Define matrices to store the converged energies and wavefunctions.
Energy_convergence_matrix = []; wf_matrix=[];
%
% \int( \bar{u}*v )dx, scalarproduct function called for at multipel places.
dotProd = @(u, v, x) sum(conj(u).*v)*dx;
%
%   Loop over the different eigenfunctions.
for wf_index=1:max_nof_wf
    %
    % Normalization of the initial wavefunction and initialization of v=du/dt.
    u = u_ini/sqrt(dotProd(u_ini,u_ini,x)); v = zeros(nof_x,1);
    %
    % Define a Lagrange multiplicator vector.
    mu = zeros(wf_index,1) ;
    %
    %  Converence criteria.
    rhs=-H*u - [wf_matrix -u]*mu - eta*v;
    convcond = sqrt(dotProd(rhs,rhs,x));
    %
    % Iteration counter for iterative solution.
```

```
iter = 1;
while convcond > tol && iter < itermax
    %
    % Define a vector for the constraints.
    G = [];
    for j=1:(wf_index-1)
        %
        % Orthogonality constraints of Eq. (19) or Eq. (A1).
        G = [G; dotProd( u, wf_matrix(:,j), x)];
    end % j
    %
    % \int( |u|^2 )dx.
    N = dotProd(u, u, x);
    %
    % Normalization constraint of Eq. (14) or Eq. (A1).
    G = [G; 1-N];
    %
    % \int( \bar{u}\hat{H}u )dx.
    E = dotProd(u, H*u, x);
    %
    % \int( |\dot{u}|^2 )dx.
    vbarv = dotProd(v, v, x);
    %
    % Explicit formula for only normalization.
    if wf_index==1
        %
        % Lagrange multiplicator for only normalization constraint, Eq. (18).
        mu = ( E + k*(1-N)/2 - vbarv )/N;
    %
    % Explicit formulae for the first excited state.
    elseif wf_index==2
        %
        % \int( u_0*\hat{H}\bar{u} )dx.
        u0Hubar = dotProd(conj(wf_matrix(:,1)), H*conj(u), x);
        %
        % \int( \bar{u}*u_0 )dx % Orthogonality constraints of Eq. (19).
        G_0 = dotProd(u, wf_matrix(:,1), x);
        %
        % Normalization constraint of Eq. (14).
        G_1 = 1 - N;
        %
        % Vector in RHS of Eq. (23).
        y_1 = k*G_0 - u0Hubar; y_2 = E - vbarv + k*G_1/2;
        %
        % \mu_0 from Eq. (24).
        mu(1) = ( (1-G_1)*y_1 + G_0*y_2)/( (1-G_1) - G_0*real(G_0) );
        %
        % \mu_1 from Eq. (24).
        mu(2) = ( y_2 + real(G_0)*y_1)/( (1-G_1) - G_0*real(G_0) );
    %
    % Works for any wf_index = 1, 2, 3, 4, ... .
    else
        %
        % Matrix in the LHS of Eq. (A6).
        M = [ eye(wf_index-1) -G(1:wf_index-1); -real(G(1:wf_index-1).') 1-G↙
```

```
(wf_index) ];
            %
            % Vector in the RHS of Eq. (A6).
            y = [ k*G(1:wf_index-1) - dotProd( conj(wf_matrix), repmat(H*conj(u),1 ,↙
wf_index-1 ), x).';
            k*G(wf_index)/2 + E - vbarv ];
            %
            % Numerical \mu-vector, see Eq. (A6).
            mu = M\y;
        end
        %v_old = v; % For standard Euler.
        % Right Hand Side of (general case) Eq. (9).
        RHS = -H*u - [wf_matrix -u]*mu - eta*v;
        %
        %  Symplectic Euler algorithms. There are two versions.
        %  Running both of them gives the famous Stormler-Verlet algorithm.
        v = v + dtau*RHS; % first
        u = u + dtau*v; % first
        %u = u + dtau*v; % second
        %v = v + dtau*(-H*u - [wf_matrix -u]*mu - eta*v); % second
        %u = u + dtau*v_old; % For standard Euler.
        %
        % Store the current value of the energy.
        Energy_convergence_matrix(iter, wf_index) = mu(wf_index);
        %
        % Convergence criteria. In this case the norm of the DFPM Eq. (12).
        convcond = sqrt(dotProd(RHS,RHS,x));
        %
        % Store the current value of the norm of the DFPM Eq. (12).
        DFPM_convergence_matrix(iter, wf_index) = convcond;
        %
        % Update counter.
        iter = iter + 1;
    end % while
    iter_record(wf_index) = iter - 1;
    %
    % Store the converged wavefunction in a matrix.
    wf_matrix(:, wf_index) = u;
end % wf_index

iter_record % Show the number of iterations for convergence.
%
% Define analytic energies.
E_analytic = [0:max_nof_wf-1]+0.5;
%
% Linewidth and fontsize for the plots below.
lw = 2; fs = 18;
%
figure; hold on
plot(x, wf_matrix + E_analytic,'linewidth',lw); plot(x, V, 'k--','linewidth',lw);
xlim([x_min x_max]); ylim([0 E_analytic(max_nof_wf)+1]); set(gca,'fontsize',fs);
ylabel('E','fontsize',fs); xlabel('x','fontsize',fs); box on
for n=0:max_nof_wf-1
    wf_analytic(n+1,:) = 1/sqrt(2^n*factorial(n))* (1/(pi))^(1/4)*hermiteH(n,x).* exp↙
(-x.^2/2); % MATLAB code.
```

```
    % wf_analytic(n+1,:) = 1/sqrt(2^n*factorial(n))* (1/(pi))^(1/4)*
    % hermitepoly(n,x).* exp(-x.^2/2);  % OCTAVE code. The miscellaneous OCTAVE↙
package must be installed.
    %
    % The prefactors of the analytic solutions compensate for the different phases↙
given by the random initial condition.
    plot(x, sign(wf_matrix(1,n+1))*sign(wf_analytic(n+1,1))*wf_analytic(n+1,:) +↙
(n+1/2),'o')
end % n
title('Eigenfunctions','fontsize',fs);
%
% For not plotting out the zeros below.
Energy_convergence_matrix( find(Energy_convergence_matrix==0) ) = NaN;
%
figure
semilogy( abs( Energy_convergence_matrix - E_analytic ),'linewidth',lw )
xlabel('Iterations','interpreter','latex','fontsize',fs); ylabel('$E_n-(n-↙
1/2)$','interpreter','latex','fontsize',fs);
set(gca,'fontsize',fs); grid
title('Convergence of energies','fontsize',fs);
%
figure
semilogy( DFPM_convergence_matrix,'linewidth',lw )
xlabel('Iterations','interpreter','latex','fontsize',fs); ylabel('$||\ddot{u}↙
||$','interpreter','latex','fontsize',fs);
set(gca,'fontsize',fs); grid
title('Convergence of the dynamical system','fontsize',fs);
%
toc
```
