# Supplementary material for: A numerical damped oscillator approach to constrained Schr\"{o}dinger equations
Source: arXiv:2002.04400 ancillary file (2020-10-20)
Supplement: Supplementary file 2 [file DFPM_1D_NLSE.pdf]

```
%
% DFPM_1D_NLSE.m % Supplemental material to M. \"{O}gren and M. Gulliksson, Eur. J.↙
Phys. 41 (2020) 065406.
% 1D Non-linear Schr\"{o}dingerequation, corresponding to \hbar=1, 2*M=1, for a ring↙
(periodic BC) with radius R=1.
%
clear all; close all
tic;
%
% Parameter for quadratic- (GPE) respectively quartic- (KSE) nonlinearity .
gamma = 7.5; kappa = 0*3;
%
% Damping parameters for DFPM and for the two constraints.
eta = 2; kvec = 1*[1;1];
%
% Define the vector with different \ell values to loop over.
ell_vector = 1e-4: 0.05: 0.99; nof_ell = length(ell_vector);
%
% Numerical tolerance and maximum number of iterations for the DFPM iteration.
tol = 1e-6; itermax = 1e4;
%
% Spatial discretization.
nof_x = 200; dx = (2*pi)/nof_x; x = (-pi:dx:(pi - dx))';
%
% Fictitious time step.
dtau = 0.95*dx;
%
% A function that returns the inner product of square integrable functions u and v.
dotProd = @(dx, u, v) sum(conj(u).*v)*dx;
%
% Initial wavefunction and initial v=du/dt for ell_index = 1. It keeps the last u, v↙
as initial conditions if ell_index > 1.
u = ( 1 + 0.01*exp(1i*x) )/sqrt(2*pi); v = zeros(nof_x,1);
%
% Loop over ell_0 values.
for ell_index = 1:nof_ell
    %
    % Present ell_0 value.
    ell_0 = ell_vector(ell_index)
    %
    % Iteration counter for iterative solution.
    convcond = Inf; iter = 1;
    while convcond > tol && iter < itermax
        %
        % Functional derivative of Eq. (33), i.e. \hat{H}u = \delta E /
        % \delta \bar{u}, see below Eq. (B10).
        Hq = -derivative(dx, derivative(dx, u,-1),1) + 2*pi*gamma*abs(u).^2.*u +↙
kappa*pi^2*abs(u).^4.*u;
        %
        % Defining the constraint functions of Eq. (34).
        G(:,1) = 1 - dotProd(dx, u, u); G(:,2) = ell_0  - dotProd(dx, u, -1↙
i*derivative(dx, u,0) );
        %
        % Define quantities needed for the Lagrange multiplicators.
        N = real(dotProd(dx, u, u));
```

```
        ell = real(dotProd(dx, -1i*derivative(dx, u, 0), u));
        E_kin = real( dotProd(dx, u, -derivative(dx, derivative(dx, u, -1), 1)) ); %↙
<u,L^2q> % = E_kin, Kinetic energy.
        %
        % Matrix M in the LHS, and vector b in the RHS of Eq. (B10).
        M = [N ell ; ell E_kin];
        b_1 = real( kvec(1)*G(1)/2 + dotProd(dx, u, Hq) - dotProd(dx, v, v) ); % Eq.↙
(B10). Only the real part is relevant since the two Lagrange multiplicators here are↙
real.
        b_2 = real( kvec(2)*G(2)/2 - 1i*dotProd(dx, conj( derivative(dx, u, 0)), conj↙
(Hq)) + 1i*dotProd(dx, v, derivative(dx, v, 0)) ); % Eq. (B10).
        %
        % Solve for the Lagrange parameters numerically.
        % mu = M\[b_1; b_2];
        %
        % Analytic formula (Cramer's rule).
        mu = ( 1/(N*E_kin-ell^2)*[ b_1*E_kin - b_2*ell ; b_2*N - b_1*ell] );
        %
        % Right Hand Side of (general case) Eq. (9), see Eq. (35).
        RHS = -Hq - [-u 1i*derivative(dx, u,0)]*mu - eta*v;
        %
        %  Symplectic Euler
        v = v + dtau*RHS;
        u = u + dtau*v;
        %
        % Calculate the distance from a solution:
        convcond = sqrt( dotProd(dx, RHS, RHS) );
        DFPM_convergence_matrix(iter, ell_index) = convcond;
        %
        % Save values of the constraints.
        G_1_convergence_matrix(iter, ell_index) = abs(G(:,1));
        G_2_convergence_matrix(iter, ell_index) = abs(G(:,2));
        %
        % Update counter.
        iter = iter + 1;
    end % while
    %
    % Shift the minimum in the densities to theta = 0.
    [~, I1] = min(abs(u).^2); I2 = nof_x/2 + 1; shift = I2 - I1; u = circshift(u,↙
shift);
    %
    % Save converged wavefunctions.
    u_sol(:, ell_index) = u;
    %
    % Save converged total energy according to Eq. (33).
    E_sol(ell_index) = E_kin + real( dotProd(dx, u, pi*gamma*abs(u).^2.*u +↙
kappa*pi^2/3*abs(u).^4.*u) );
    %
    % Save converged Lagrange multiplicators.
    chmPotsol(ell_index) = mu(1); angVelsol(ell_index) = mu(2);
    %
end % ell_index
%
% Fontsize, linewidth, and markersize, for the plots.
fs = 20; lw = 2; ms = 10; % Fontsize, linewidth, and markersize, for the plots.
```

```
%
% Plot figures.
figure
subplot(2,1,1); plot(x,abs(u_sol).^2,'linewidth',lw); xlim([-pi pi]) % Density.
set(gca,'fontsize',fs,'XTickLabel',{}); ylabel('|u|^2','fontsize',fs); box on
title('Density and phase of the wavefunctions','fontsize',fs)
%
subplot(2,1,2); plot(x,angle(u_sol),'linewidth',lw); axis([-pi pi -pi pi]) % Phase.
xlabel('x','fontsize',fs); ylabel('phase(u)','fontsize',fs); box on
set(gca,'fontsize',fs,'xtick',[-pi 0 pi],'XTickLabel',{'-\pi','0','\pi'},'Ytick',[-pi↙
0 pi],'YTickLabel',{'-\pi','0','\pi'})
%
figure;
for ell_index=1:nof_ell
    semilogy(DFPM_convergence_matrix(:, ell_index),'linewidth',lw), hold on; %↙
Convergence.
end % ell_index
grid on; xlabel('Iterations'); ylabel('$||\ddot{u}↙
||$','interpreter','latex','fontsize',fs); box on
title('Convergence.','fontsize',fs)
%
figure;
for ell_index=1:nof_ell
    subplot(2,1,1); semilogy(G_1_convergence_matrix(:, ell_index),'linewidth',lw),↙
hold on; % Convergence of G_1.
    subplot(2,1,2); semilogy(G_2_convergence_matrix(:, ell_index),'linewidth',lw),↙
hold on; % Convergence of G_2.
end % ell_index
grid on; xlabel('Iterations'); ylabel('$|G_{2}|$','interpreter','latex','fontsize',↙
fs); box on
subplot(2,1,1); ylabel('$|G_{1}|$','interpreter','latex','fontsize',fs); box on
title('Convergence of constraints.','fontsize',fs)
%
figure; hold on
plot(ell_vector, E_sol,'b.-','MarkerSize',ms), grid on
plot(0, gamma/2,'ro'); plot(1, gamma/2+1,'ro') % GPE reference values for plane-waves↙
solutions.
%plot(0, kappa/12,'ro'); plot(1, kappa/12+1,'ro') % KSE reference values for plane-↙
waves solutions.
ylabel('$E$','Interpreter','latex','fontsize',fs); xlabel↙
('$\ell$','Interpreter','latex','fontsize',fs); box on
title('Yrast curve','fontsize',fs)
%
figure
subplot(2,1,1); plot(ell_vector,chmPotsol,'b.-','MarkerSize',ms) % The chemical↙
potential \mu is one of the Lagrange multiplicators.
ylabel('\mu','fontsize',fs); box on
title('Lagrange multiplicators','fontsize',fs)
%
subplot(2,1,2); plot(ell_vector,angVelsol,'r.-','MarkerSize',ms) % The angular↙
velocity \Omega is one of the Lagrange multiplicators.
xlabel('$\ell$','Interpreter','latex','fontsize',fs); ylabel('\Omega','fontsize',fs);↙
box on
toc
%
```

```
% Calculating first order derivatives.
% For OCTAVE, copy the following function in a file called "derivative.m" and place it↙
in the same folder as this file (DFPM_1D_NLSE.m).
% For MATLAB, leave this function here.
function [ dq ] = derivative(h, u, BCF)
    if BCF == -1 % Backward.
        dq = (circshift(u, -1) - circshift(u, 0))/(h);
    elseif BCF == 0 % Central.
        dq = (circshift(u, -1) - circshift(u, 1))/(2*h);
    elseif BCF == 1 % Forward.
        dq = (circshift(u, 0) - circshift(u, 1))/(h);
    end
end
%
```
